# Supplementary material for: Development and analysis of a Bayesian water balance model for large lake systems
Source: arXiv:1710.10161 ancillary file (2018-05-16)
Supplement: Supplementary file 1 [file glwb_model_improve_si.pdf]

# Supplementary Material: Development and analysis of a Bayesian water balance model for large lake systems

Joeseph P. Smith[a], Andrew D. Gronewold[b,c]

[a]Cooperative Institute for Great Lakes Research, University of Michigan, Ann Arbor, Michigan USA, 48109
[b]Great Lakes Environmental Research Laboratory, National Oceanic and Atmospheric Administration, Ann Arbor, Michigan, USA, 48108
[c]Department of Civil and Environmental Engineering, University of Michigan, Ann Arbor, Michigan USA, 48109

## 1. Contents

- Page 3 - Prior distributions for Lake Superior's water balance components
- Page 4 - Prior distributions for Lake Michigan-Huron's water balance components
- Page 5 - Prototype model posterior inferences for Lake Superior's water balance components
- Page 6 - Prototype model posterior inferences for Lake Michigan-Huron's water balance components
- Page 7 - f12NF model posterior inferences for Lake Superior's water balance components
- Page 8 - f12NF model posterior inferences for Lake Michigan-Huron's water balance components
- Page 9 - f12FF model posterior inferences for Lake Superior's water balance components

*Corresponding author. Tel.: +1-734-741-2252, Fax: +1 734-741-2055
*Email address:* joeseph@umich.edu (Joeseph P. Smith)

- Page 10 - f12FF model posterior inferences for Lake Michigan-Huron's water balance components
- Pages 12-17: (f)XXFF model BUGS code
- Pages 18-24: (f)XXHH model BUGS code

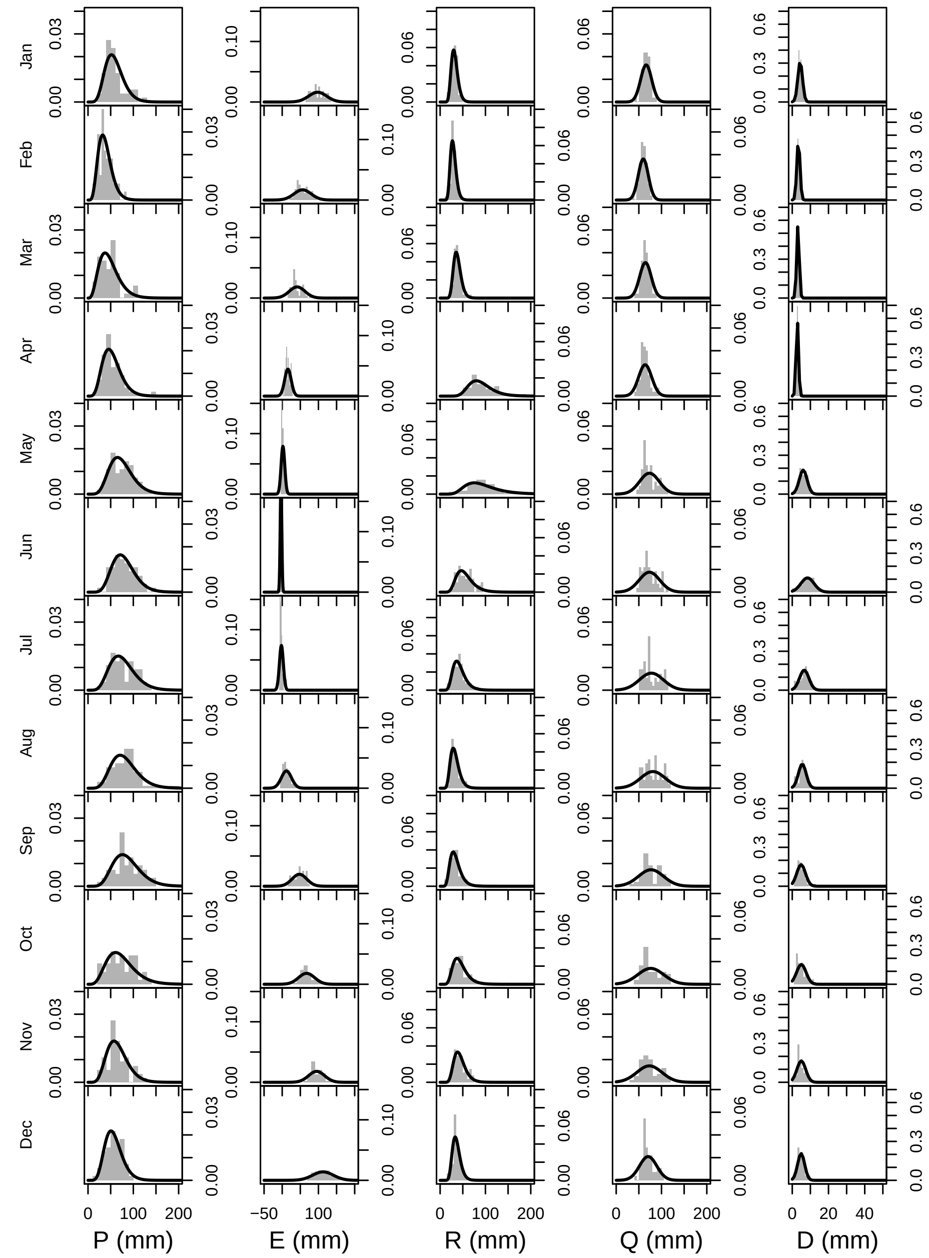


Figure 1: Prior distributions as described in section 2.3.1 for water balance components on Lake Superior. Unbordered gray rectangles in the background are histograms of the historical record (1950-2004) from the NOAA-GLERL GLM-HMD and coordinated estimates. Solid lines represent our informative prior distributions.

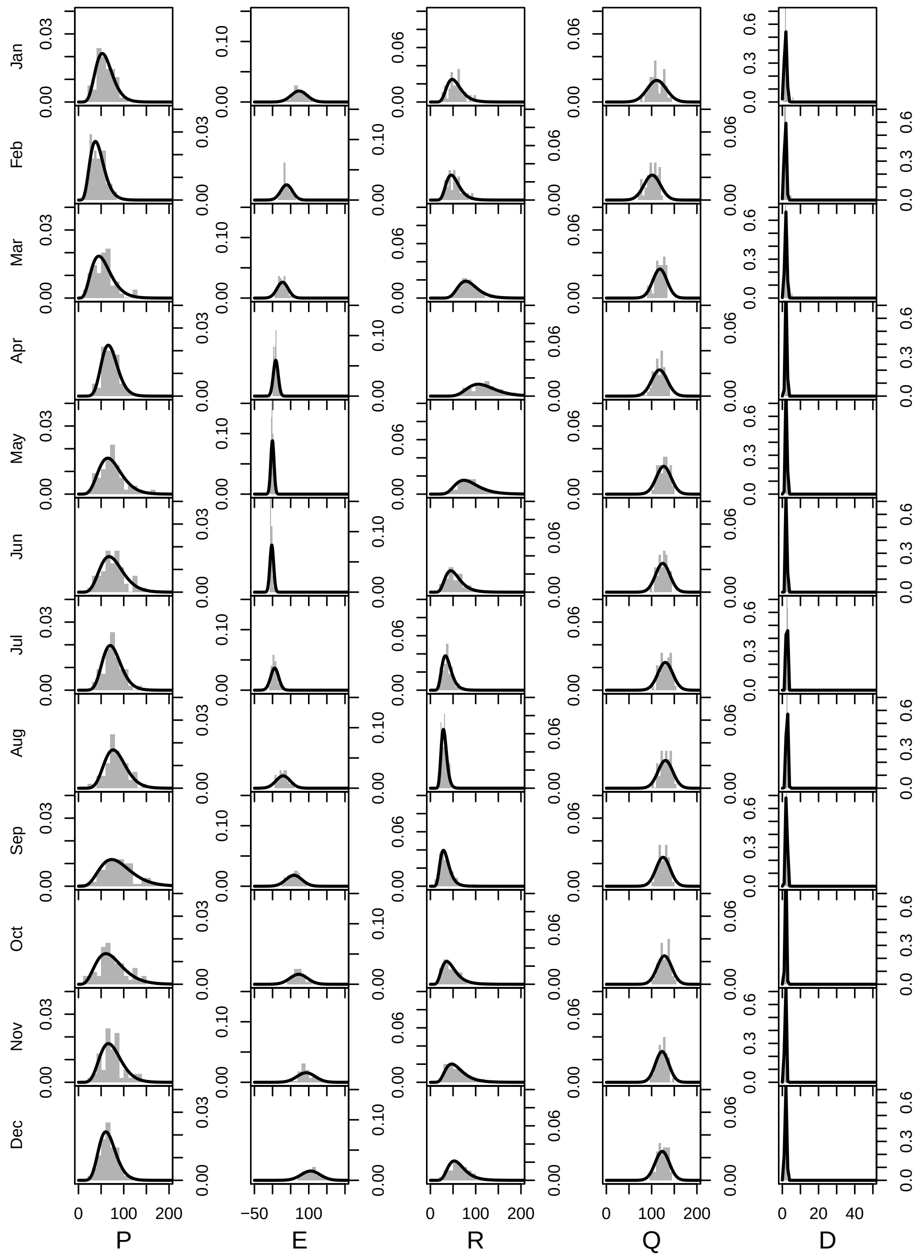


Figure 2: Prior distributions as described in section 2.3.1 for water balance components on Lake Michigan-Huron. Unbordered gray rectangles in the background are histograms of the historical record (1950-2004) from the NOAA-GLERL GLM-HMD and coordinated estimates. Solid lines represent our informative prior distributions.

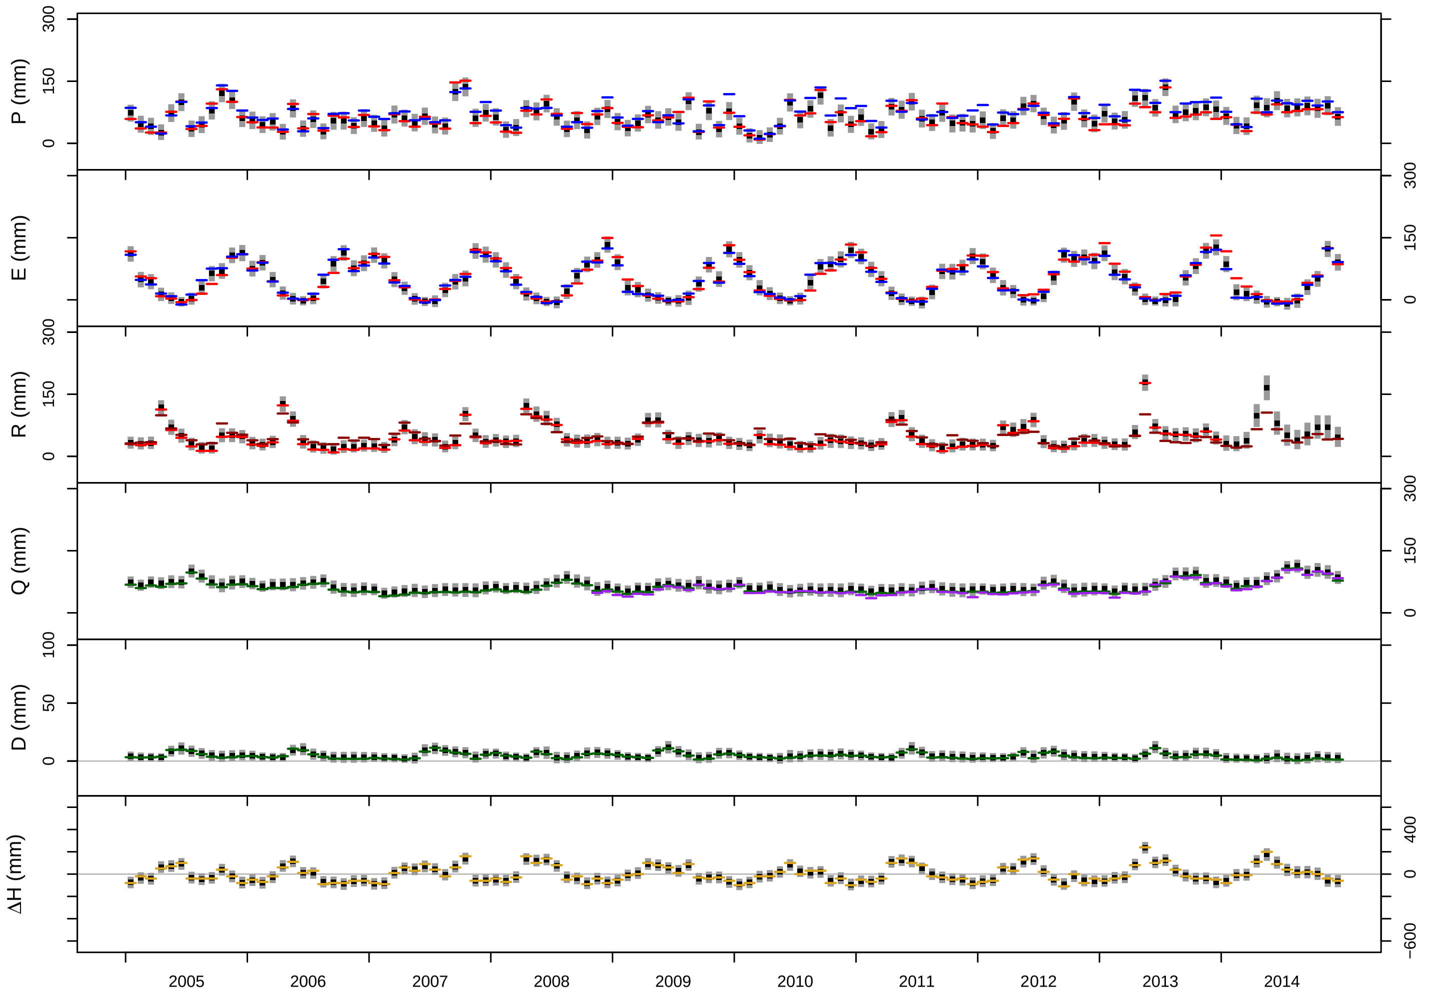


Figure 3: Posterior inferences (gray bars indicate 95% credible intervals, with black squares for the median estimates) from the prototype model for Lake Superior's water balance components. For P and E, the red segments represent data from the NOAA-GLERL GLM-HMD, and the blue segments from CaPA and GEM-MESH. For R, red segments also represent the GLM-HMD, and the darker red segments represent the NOAA-GLERL LBRM. For Q and D, the green segments are coordinated estimates, purple segments for international gauging stations (IGS). For $\Delta H$, the gold segments represent coordinated estimates of month-to-month change in storage, or $y_{SUP,\Delta H,t,1}$ while gray bars represent the posterior predictive distributions for those estimates.

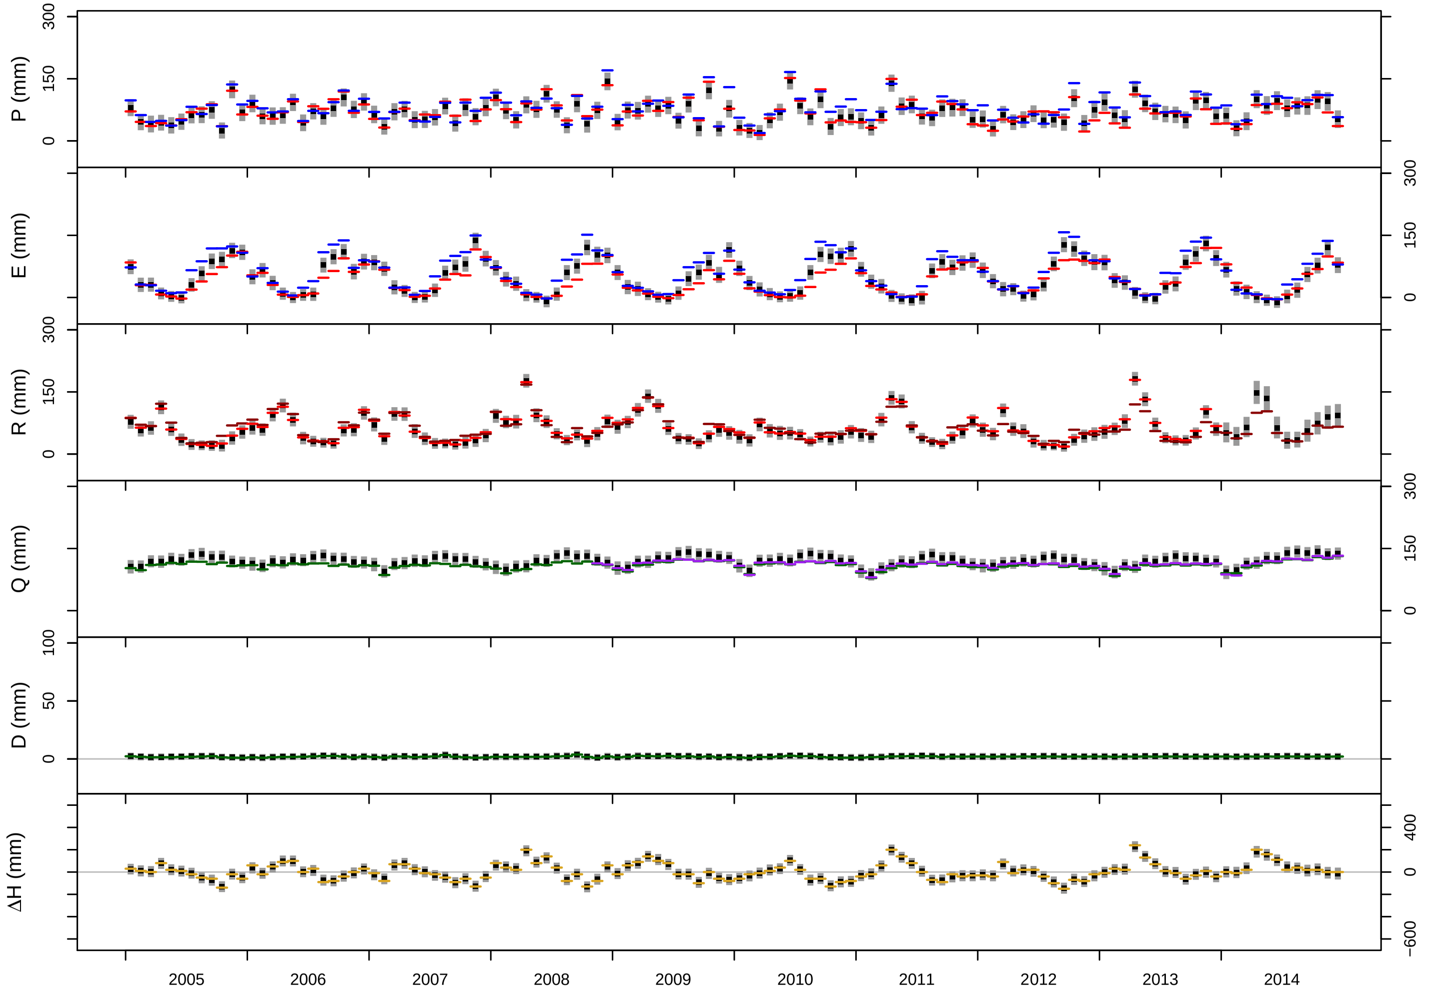


Figure 4: Posterior inferences (gray bars indicate 95% credible intervals, with black squares for the median estimates) from the prototype model for Lake Michigan-Huron's water balance components. For P and E, the red segments represent data from the NOAA-GLERL GLM-HMD, and the blue segments from CaPA and GEM-MESH. For R, red segments also represent the GLM-HMD, and the darker red segments represent the NOAA-GLERL LBRM. For Q and D, the green segments are coordinated estimates, purple segments for international gauging stations (IGS). For $\Delta H$, the gold segments represent coordinated estimates of month-to-month change in storage, or $y_{MHU,\Delta H,t,1}$ while gray bars represent the posterior predictive distributions for those estimates.

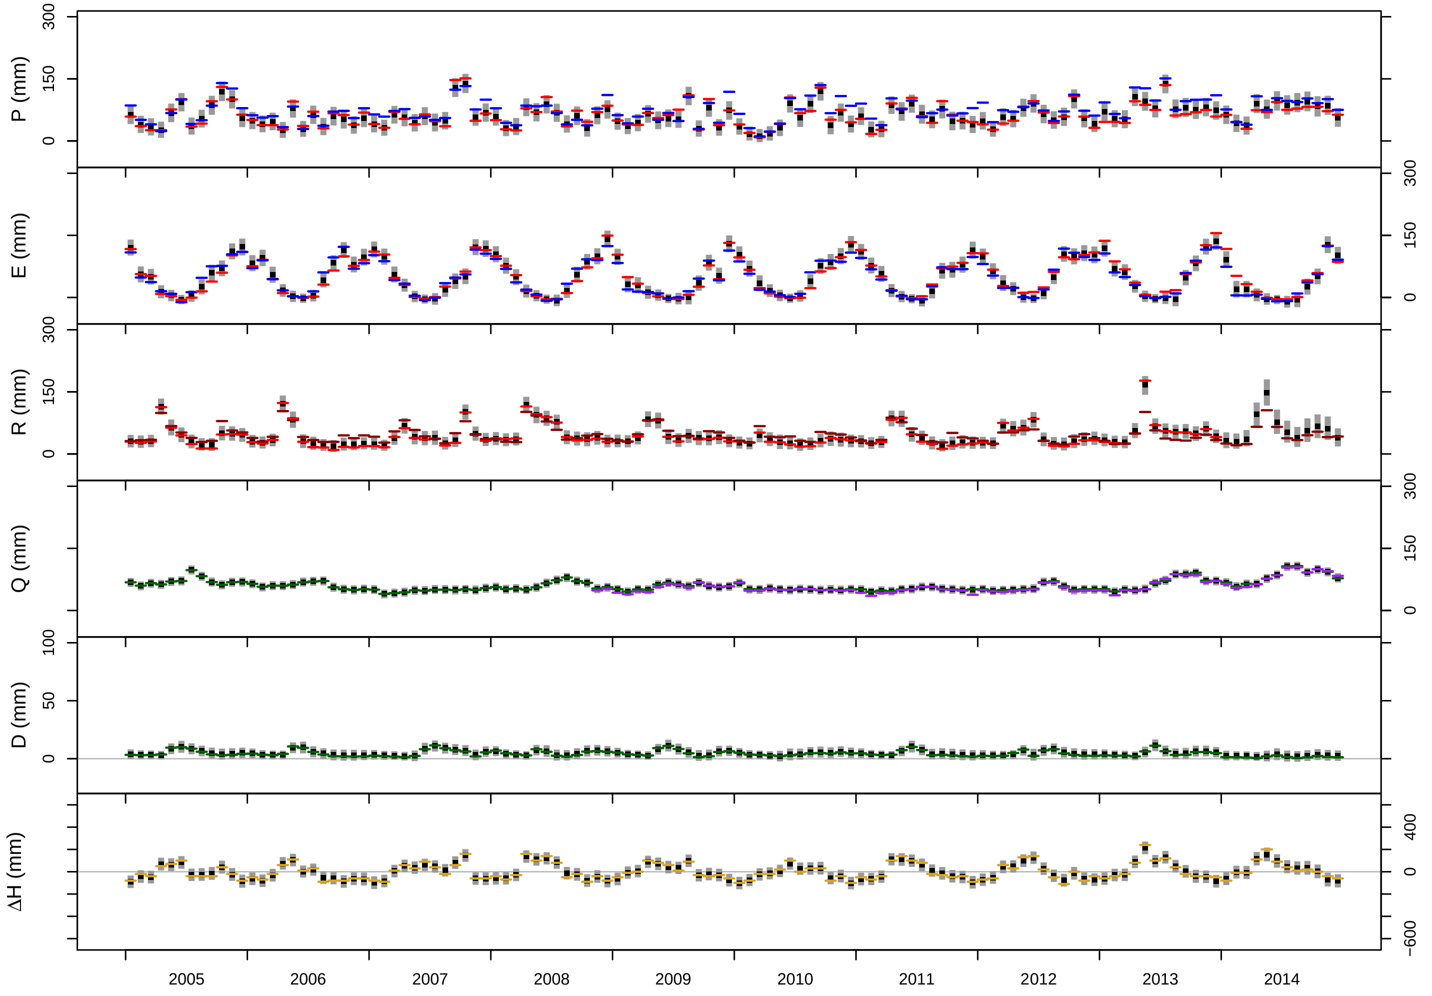


Figure 5: Posterior inferences (gray bars indicate 95% credible intervals, with black squares for the median estimates) from the f12NF model for Lake Superior's water balance components. For P and E, the red segments represent data from the NOAA-GLERL GLM-HMD, and the blue segments from CaPA and GEM-MESH. For R, red segments also represent the GLM-HMD, and the darker red segments represent the NOAA-GLERL LBRM. For Q and D, the green segments are coordinated estimates, purple segments for international gauging stations (IGS). For $\Delta H$, the gold segments represent coordinated estimates of month-to-month change in storage, or $y_{SUP,\Delta H,t,1}$ while gray bars represent the posterior predictive distributions for those estimates.

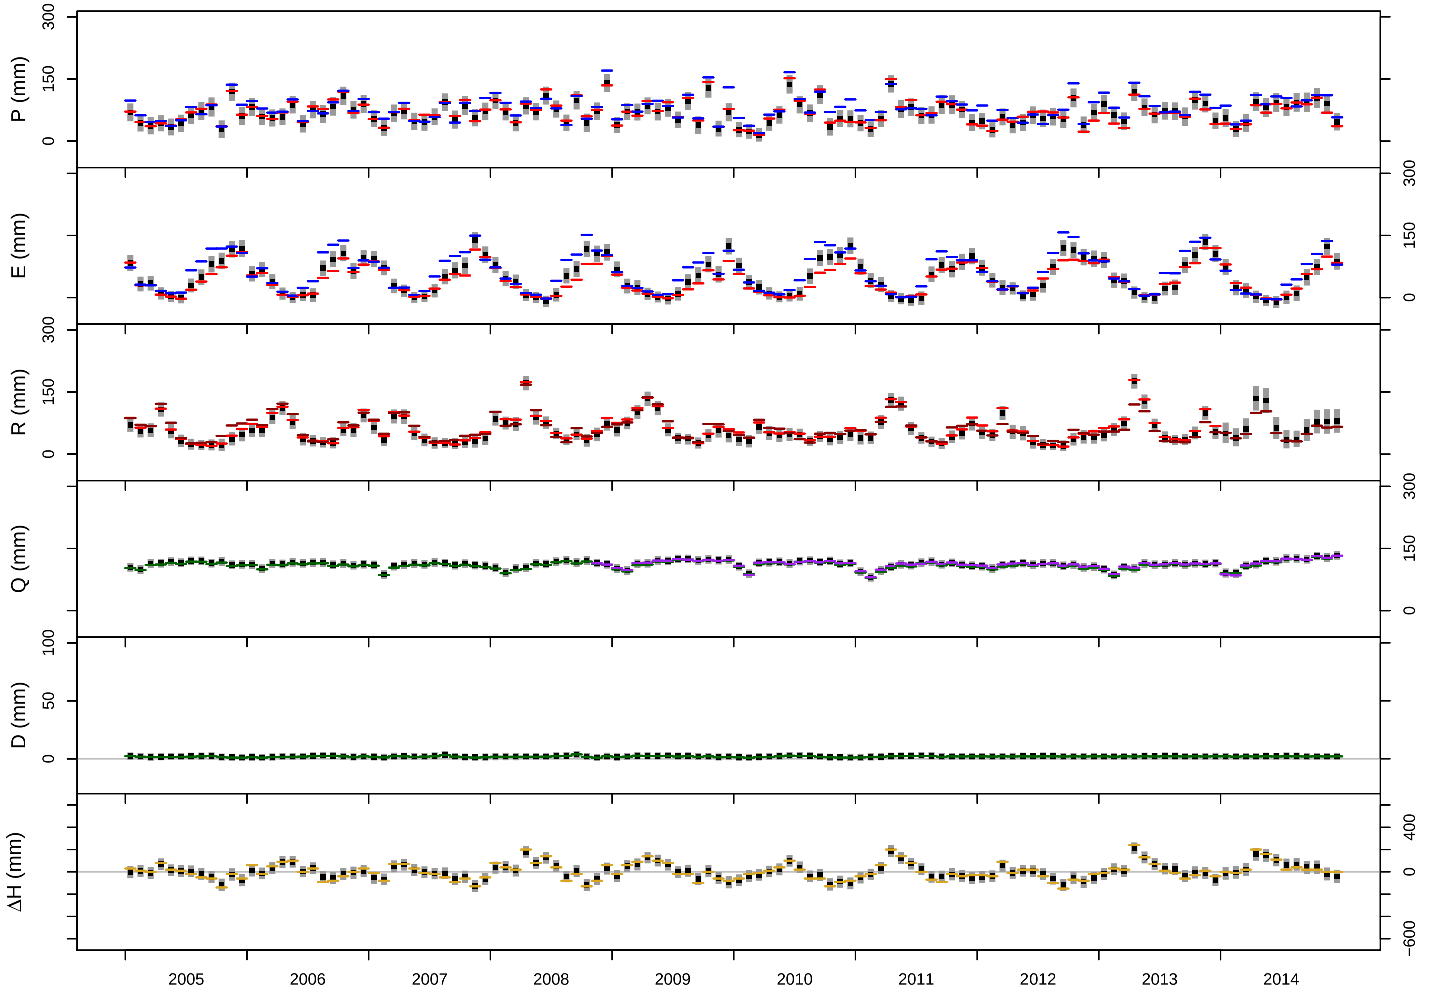


Figure 6: Posterior inferences (gray bars indicate 95% credible intervals, with black squares for the median estimates) from the f12NF model for Lake Michigan-Huron's water balance components. For P and E, the red segments represent data from the NOAA-GLERL GLM-HMD, and the blue segments from CaPA and GEM-MESH. For R, red segments also represent the GLM-HMD, and the darker red segments represent the NOAA-GLERL LBRM. For Q and D, the green segments are coordinated estimates, purple segments for international gauging stations (IGS). For $\Delta H$, the gold segments represent coordinated estimates of month-to-month change in storage, or $y_{MHU,\Delta H,t,1}$ while gray bars represent the posterior predictive distributions for those estimates.

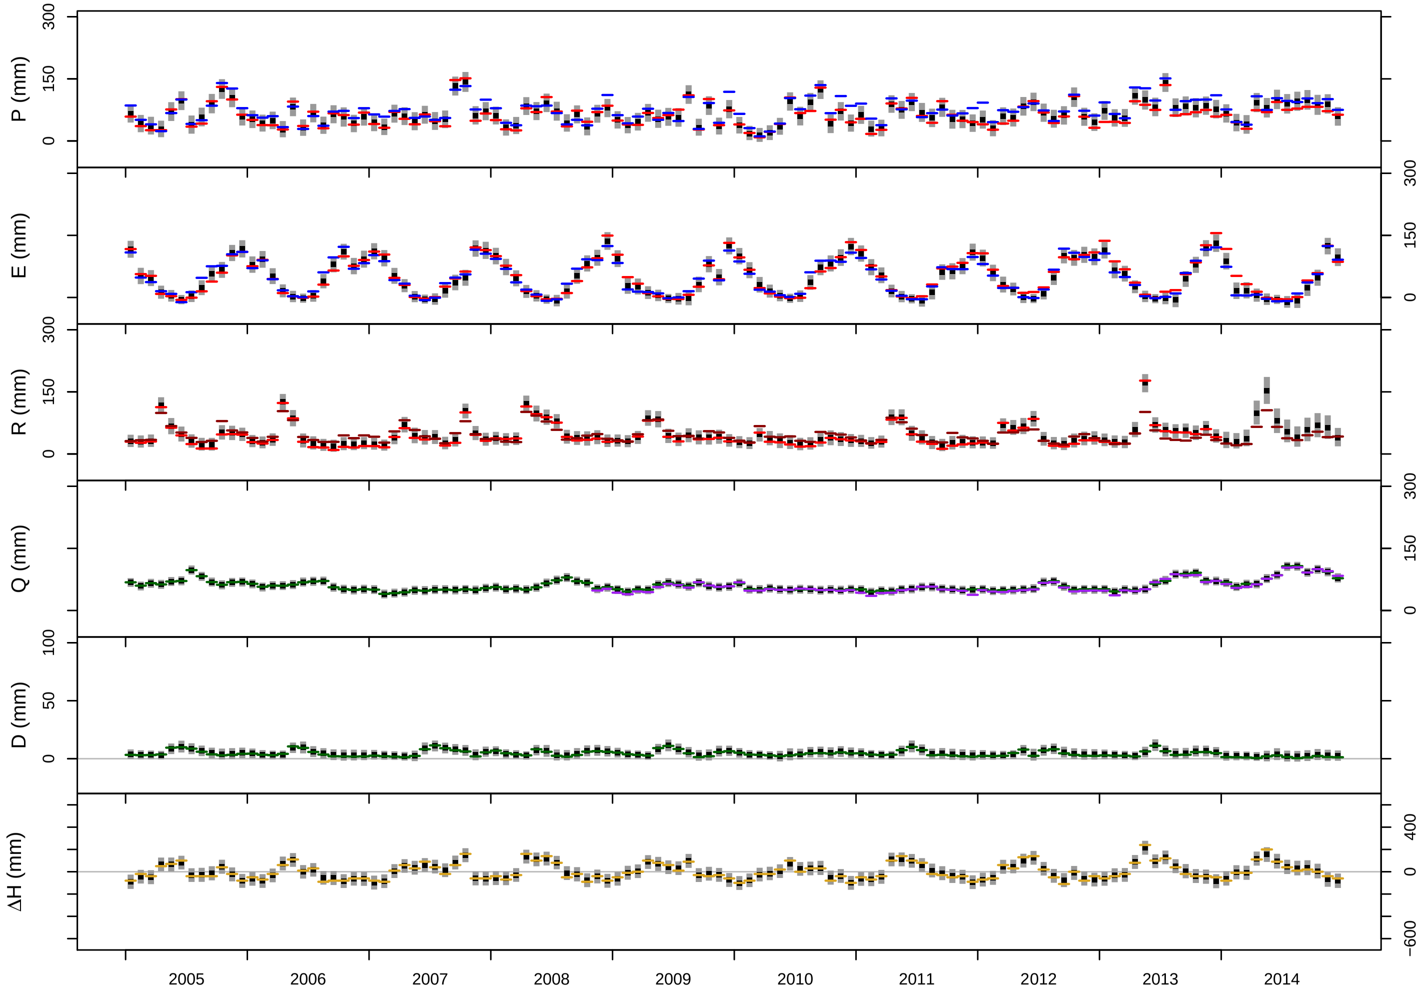


Figure 7: Posterior inferences (gray bars indicate 95% credible intervals, with black squares for the median estimates) from the f12FF model for Lake Superior's water balance components. For P and E, the red segments represent data from the NOAA-GLERL GLM-HMD, and the blue segments from CaPA and GEM-MESH. For R, red segments also represent the GLM-HMD, and the darker red segments represent the NOAA-GLERL LBRM. For Q and D, the green segments are coordinated estimates, purple segments for international gauging stations (IGS). For $\Delta H$, the gold segments represent coordinated estimates of month-to-month change in storage, or $y_{SUP,\Delta H,t,1}$ while gray bars represent the posterior predictive distributions for those estimates.

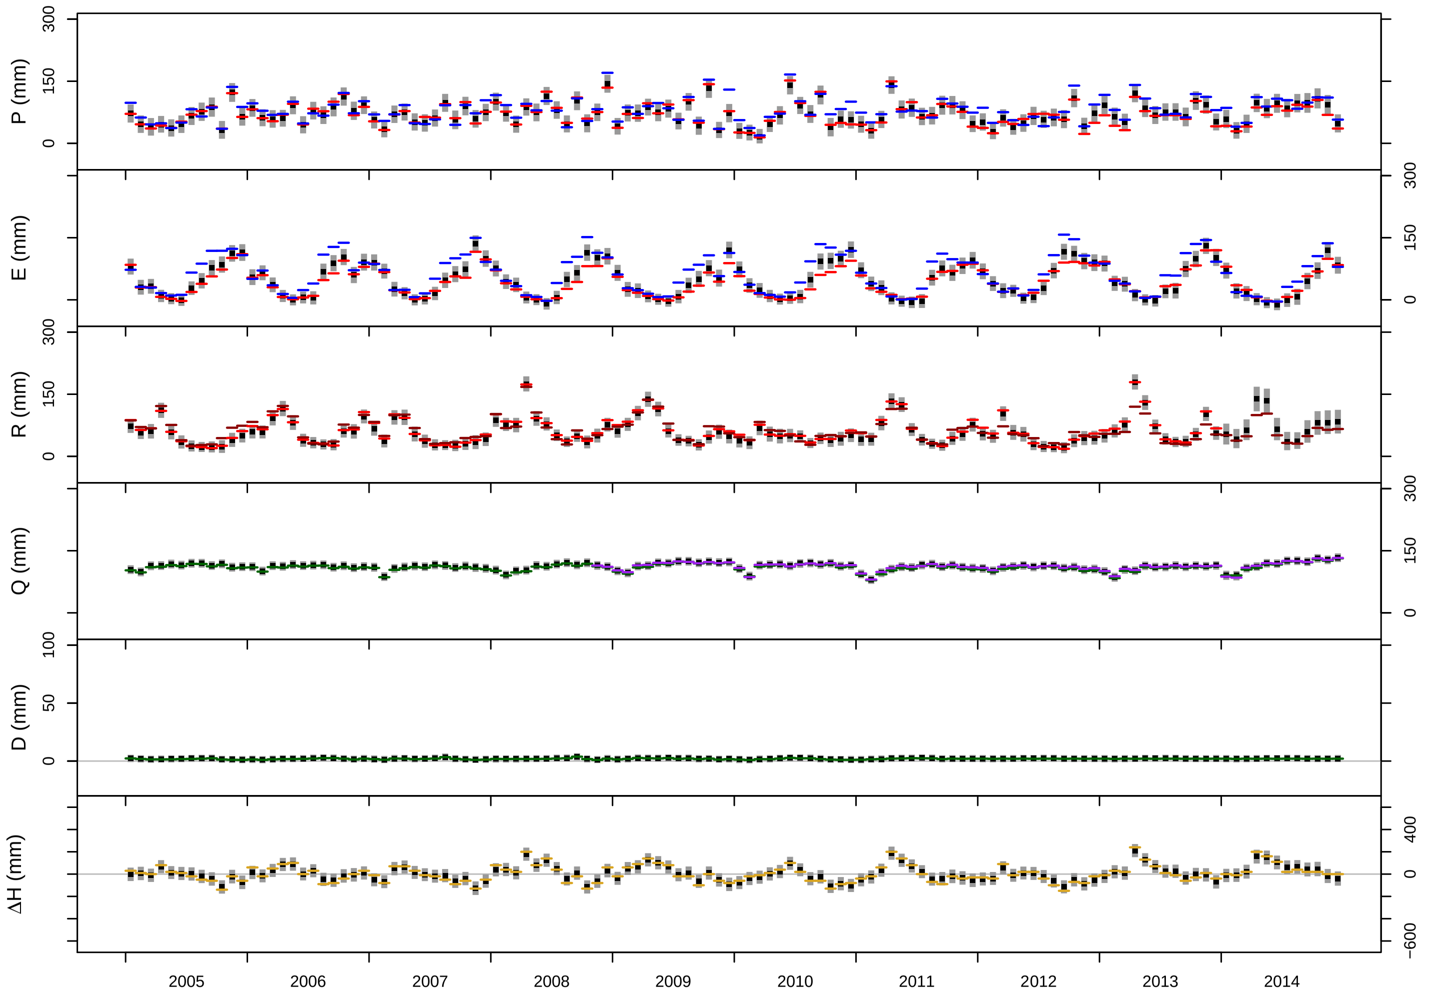


Figure 8: Posterior inferences (gray bars indicate 95% credible intervals, with black squares for the median estimates) from the f12FF model for Lake Michigan-Huron's water balance components. For P and E, the red segments represent data from the NOAA-GLERL GLM-HMD, and the blue segments from CaPA and GEM-MESH. For R, red segments also represent the GLM-HMD, and the darker red segments represent the NOAA-GLERL LBRM. For Q and D, the green segments are coordinated estimates, purple segments for international gauging stations (IGS). For $\Delta H$, the gold segments represent coordinated estimates of month-to-month change in storage, or $y_{MHU,\Delta H,t,1}$ while gray bars represent the posterior predictive distributions for those estimates.

MODEL CODE

```
### (f)12FF MODEL WITH POSTERIOR PREDICTIVE DISTRIBUTIONS FOR ALL VARIABLES

model {
    for (j in posteriorStartMonth:posteriorEndMonth){

        ##########################################
        ## Priors as described in section 2.2.2
        ## Data are fed in through R in jags.model
        ## function call, via data parameter
        ## Note: distribution parameters are
        ## mean and precision
        ## precision = 1/variance
        ##########################################

        ### SUPERIOR
        superiorPrecip[j] ~ dgamma(superiorPriorPrecipShape[m[j]], superiorPriorPrecipRate[m[j]])
        superiorEvap[j] ~ dnorm(superiorEvapPriorMean[m[j]], superiorEvapPriorPrecision[m[j]])
        superiorRunoff[j]   <- exp(superiorLogRunoff[j])
        superiorLogRunoff[j] ~ dnorm(superiorRunoffLogPriorMean[m[j]], superiorRunoffLogPriorPrecision[m[j]])
        superiorOutflow[j] ~ dnorm(superiorOutflowPriorMean[m[j]], superiorOutflowPriorPrecision[m[j]])
        superiorDiversion[j] ~ dnorm(superiorDiversionPriorMean[m[j]], superiorDiversionPriorPrecision[m[j]])


        ### MICHIGAN-HURON
        miHuronPrecip[j]    ~ dgamma(miHuronPriorPrecipShape[m[j]], miHuronPriorPrecipRate[m[j]])
        miHuronEvap[j] ~ dnorm(miHuronEvapPriorMean[m[j]], miHuronEvapPriorPrecision[m[j]])
        miHuronRunoff[j]    <- exp(miHuronLogRunoff[j])
        miHuronLogRunoff[j] ~ dnorm(miHuronRunoffLogPriorMean[m[j]], miHuronRunoffLogPriorPrecision[m[j]])
        miHuronOutflow[j] ~ dnorm(miHuronOutflowPriorMean[m[j]], miHuronOutflowPriorPrecision[m[j]])
        miHuronDiversion[j] ~ dnorm(miHuronDiversionPriorMean[m[j]], miHuronDiversionPriorPrecision[m[j]])

        ########################################################
        ## Likelihood functions as described in section 2.2.2
        ## Biases follow equation 6
        ########################################################

        ### SUPERIOR
        ySuperiorPrecip1[j] ~ dnorm(ySuperiorPrecip1Mean[j], ySuperiorPrecip1Prec)
        ySuperiorPrecip2[j] ~ dnorm(ySuperiorPrecip2Mean[j], ySuperiorPrecip2Prec)
        ySuperiorEvap1[j] ~ dnorm(ySuperiorEvap1Mean[j], ySuperiorEvap1Prec)
        ySuperiorEvap2[j] ~ dnorm(ySuperiorEvap2Mean[j], ySuperiorEvap2Prec)
        ySuperiorRunoff1[j] ~ dnorm(ySuperiorRunoff1Mean[j], ySuperiorRunoff1Prec)
        ySuperiorRunoff2[j] ~ dnorm(ySuperiorRunoff2Mean[j], ySuperiorRunoff2Prec)
        ySuperiorOutflow1[j]  ~ dnorm(ySuperiorOutflow1Mean[j], ySuperiorOutflow1Prec)
        ySuperiorOutflow2[j]  ~ dnorm(ySuperiorOutflow2Mean[j], ySuperiorOutflow2Prec)
        ySuperiorDiversion1[j]  ~ dnorm(ySuperiorDiversion1Mean[j], ySuperiorDiversion1Prec)

        ySuperiorPrecip1Mean[j] <- superiorPrecip[j] + ySuperiorPrecip1Bias[m[j]]
        ySuperiorPrecip2Mean[j] <- superiorPrecip[j] + ySuperiorPrecip2Bias[m[j]]
        ySuperiorEvap1Mean[j] <- superiorEvap[j] + ySuperiorEvap1Bias[m[j]]
        ySuperiorEvap2Mean[j] <- superiorEvap[j] + ySuperiorEvap2Bias[m[j]]
        ySuperiorRunoff1Mean[j] <- superiorRunoff[j] + ySuperiorRunoff1Bias[m[j]]
        ySuperiorRunoff2Mean[j] <- superiorRunoff[j] + ySuperiorRunoff2Bias[m[j]]
        ySuperiorOutflow1Mean[j] <- superiorOutflow[j] + ySuperiorOutflow1Bias[m[j]]
        ySuperiorOutflow2Mean[j] <- superiorOutflow[j] + ySuperiorOutflow2Bias[m[j]]
        ySuperiorDiversion1Mean[j] <- superiorDiversion[j] + ySuperiorDiversion1Bias[m[j]]
```

```
    ### MICHIGAN-HURON
    yMiHuronPrecip1[j] ~ dnorm(yMiHuronPrecip1Mean[j], yMiHuronPrecip1Prec)
    yMiHuronPrecip2[j] ~ dnorm(yMiHuronPrecip2Mean[j], yMiHuronPrecip2Prec)
    yMiHuronEvap1[j] ~ dnorm(yMiHuronEvap1Mean[j], yMiHuronEvap1Prec)
    yMiHuronEvap2[j] ~ dnorm(yMiHuronEvap2Mean[j], yMiHuronEvap2Prec)
    yMiHuronRunoff1[j] ~ dnorm(yMiHuronRunoff1Mean[j], yMiHuronRunoff1Prec)
    yMiHuronRunoff2[j] ~ dnorm(yMiHuronRunoff2Mean[j], yMiHuronRunoff2Prec)
    yMiHuronOutflow1[j]  ~ dnorm(yMiHuronOutflow1Mean[j], yMiHuronOutflow1Prec)
    yMiHuronOutflow2[j]  ~ dnorm(yMiHuronOutflow2Mean[j], yMiHuronOutflow2Prec)
    yMiHuronDiversion1[j]  ~ dnorm(yMiHuronDiversion1Mean[j], yMiHuronDiversion1Prec)

    yMiHuronPrecip1Mean[j] <- miHuronPrecip[j] + yMiHuronPrecip1Bias[m[j]]
    yMiHuronPrecip2Mean[j] <- miHuronPrecip[j] + yMiHuronPrecip2Bias[m[j]]
    yMiHuronEvap1Mean[j] <- miHuronEvap[j] + yMiHuronEvap1Bias[m[j]]
    yMiHuronEvap2Mean[j] <- miHuronEvap[j] + yMiHuronEvap2Bias[m[j]]
    yMiHuronRunoff1Mean[j] <- miHuronRunoff[j] + yMiHuronRunoff1Bias[m[j]]
    yMiHuronRunoff2Mean[j] <- miHuronRunoff[j] + yMiHuronRunoff2Bias[m[j]]
    yMiHuronOutflow1Mean[j] <- miHuronOutflow[j] + yMiHuronOutflow1Bias[m[j]]
    yMiHuronOutflow2Mean[j] <- miHuronOutflow[j] + yMiHuronOutflow2Bias[m[j]]
    yMiHuronDiversion1Mean[j] <- miHuronDiversion[j] + yMiHuronDiversion1Bias[m[j]]

}

#####################################################
# Water balance model as described in section 2.1
# Model/Process error follows equation 4
#####################################################

for(k in rollPeriod:posteriorEndMonth){
    ### SUPERIOR
    ySuperiorRStore[k] ~ dnorm(superiorRStore[k], ySuperiorRStorePrec)

    superiorRStore[k] <- (
        sum(superiorPrecip[(k-rollPeriod+1):k])
        -sum(superiorEvap[(k-rollPeriod+1):k])
        +sum(superiorRunoff[(k-rollPeriod+1):k])
        -sum(superiorOutflow[(k-rollPeriod+1):k])
        +sum(superiorDiversion[(k-rollPeriod+1):k])
        +sum(superiorProcError[m[(k-rollPeriod+1):k]])
    )

    ### MICHIGAN-HURON
    yMiHuronRStore[k] ~ dnorm(miHuronRStore[k], yMiHuronRStorePrec)

    miHuronRStore[k] <- (
        sum(miHuronPrecip[(k-rollPeriod+1):k])
        -sum(miHuronEvap[(k-rollPeriod+1):k])
        +sum(miHuronRunoff[(k-rollPeriod+1):k])
        -sum(miHuronOutflow[(k-rollPeriod+1):k])
        +0.70110653739*sum(superiorOutflow[(k-rollPeriod+1):k])
        -sum(miHuronDiversion[(k-rollPeriod+1):k])
```

```
        +sum(miHuronProcError[m[(k-rollPeriod+1):k]])
    )
}

####################################################################
## Bias terms and process errors, equations 4 and 6 respectively
## Includes incorporation of expert guidance on Q and D
## They would otherwise have the same bias definition as the other
## variables
####################################################################
for (i in 1:12){
    ySuperiorPrecip1Bias[i] ~ dnorm(0,0.01)
    ySuperiorPrecip2Bias[i] ~ dnorm(0,0.01)
    ySuperiorEvap1Bias[i] ~ dnorm(0,0.01)
    ySuperiorEvap2Bias[i] ~ dnorm(0,0.01)
    ySuperiorRunoff1Bias[i] ~ dnorm(0,0.01)
    ySuperiorRunoff2Bias[i] ~ dnorm(0,0.01)
    ySuperiorOutflow1Bias[i] ~ dnorm(0,0.25)
    ySuperiorOutflow2Bias[i] ~ dnorm(0,0.25)
    ySuperiorDiversion1Bias[i] ~ dnorm(0,0.25)

    yMiHuronPrecip1Bias[i] ~ dnorm(0,0.01)
    yMiHuronPrecip2Bias[i] ~ dnorm(0,0.01)
    yMiHuronEvap1Bias[i] ~ dnorm(0,0.01)
    yMiHuronEvap2Bias[i] ~ dnorm(0,0.01)
    yMiHuronRunoff1Bias[i] ~ dnorm(0,0.01)
    yMiHuronRunoff2Bias[i] ~ dnorm(0,0.01)
    yMiHuronOutflow1Bias[i] ~ dnorm(0,0.25)
    yMiHuronOutflow2Bias[i] ~ dnorm(0,0.25)
    yMiHuronDiversion1Bias[i] ~ dnorm(0,0.25)

    superiorProcError[i] ~ dnorm(0,0.01)
    miHuronProcError[i] ~ dnorm(0,0.01)
}

##############################
## Precision for Observations
##############################

### SUPERIOR
ySuperiorRStorePrec    ~ dgamma(0.01,0.01)
ySuperiorPrecip1Prec   ~ dgamma(0.1,0.1)
ySuperiorPrecip2Prec   ~ dgamma(0.1,0.1)
ySuperiorEvap1Prec     ~ dgamma(0.1,0.1)
ySuperiorEvap2Prec     ~ dgamma(0.1,0.1)
ySuperiorRunoff1Prec   ~ dgamma(0.1,0.1)
ySuperiorRunoff2Prec   ~ dgamma(0.1,0.1)
ySuperiorOutflow1Prec ~ dgamma(0.1,0.1)
ySuperiorOutflow2Prec ~ dgamma(0.1,0.1)
ySuperiorDiversion1Prec ~ dgamma(0.1,0.1)

### MICHIGAN-HURON
yMiHuronRStorePrec ~ dgamma(0.01,0.01)
yMiHuronPrecip1Prec ~ dgamma(0.1,0.1)
yMiHuronPrecip2Prec ~ dgamma(0.1,0.1)
yMiHuronEvap1Prec ~ dgamma(0.1,0.1)
yMiHuronEvap2Prec ~ dgamma(0.1,0.1)
```

```
yMiHuronRunoff1Prec ~ dgamma(0.1,0.1)
yMiHuronRunoff2Prec ~ dgamma(0.1,0.1)
yMiHuronOutflow1Prec ~ dgamma(0.1,0.1)
yMiHuronOutflow2Prec ~ dgamma(0.1,0.1)
yMiHuronDiversion1Prec ~ dgamma(0.1,0.1)




##################################################################
# Posterior predictive (PP) distributions for verification
##################################################################

for(jp in posteriorStartMonth:posteriorEndMonth){
    ### SUPERIOR
    ySuperiorPrecip1PP[jp] ~ dnorm(ySuperiorPrecip1Mean[jp], ySuperiorPrecip1Prec)
    ySuperiorPrecip2PP[jp] ~ dnorm(ySuperiorPrecip2Mean[jp], ySuperiorPrecip2Prec)
    ySuperiorEvap1PP[jp] ~ dnorm(ySuperiorEvap1Mean[jp], ySuperiorEvap1Prec)
    ySuperiorEvap2PP[jp] ~ dnorm(ySuperiorEvap2Mean[jp], ySuperiorEvap2Prec)
    ySuperiorRunoff1PP[jp] ~ dnorm(ySuperiorRunoff1Mean[jp], ySuperiorRunoff1Prec)
    ySuperiorRunoff2PP[jp] ~ dnorm(ySuperiorRunoff2Mean[jp], ySuperiorRunoff2Prec)
    ySuperiorOutflow1PP[jp] ~ dnorm(ySuperiorOutflow1Mean[jp], ySuperiorOutflow1Prec)
    ySuperiorOutflow2PP[jp] ~ dnorm(ySuperiorOutflow2Mean[jp], ySuperiorOutflow2Prec)
    ySuperiorDiversion1PP[jp] ~ dnorm(ySuperiorDiversion1Mean[jp], ySuperiorDiversion1Prec)

    ### MICHIGAN-HURON
    yMiHuronPrecip1PP[jp] ~ dnorm(yMiHuronPrecip1Mean[jp], yMiHuronPrecip1Prec)
    yMiHuronPrecip2PP[jp] ~ dnorm(yMiHuronPrecip2Mean[jp], yMiHuronPrecip2Prec)
    yMiHuronEvap1PP[jp] ~ dnorm(yMiHuronEvap1Mean[jp], yMiHuronEvap1Prec)
    yMiHuronEvap2PP[jp] ~ dnorm(yMiHuronEvap2Mean[jp], yMiHuronEvap2Prec)
    yMiHuronRunoff1PP[jp] ~ dnorm(yMiHuronRunoff1Mean[jp], yMiHuronRunoff1Prec)
    yMiHuronRunoff2PP[jp] ~ dnorm(yMiHuronRunoff2Mean[jp], yMiHuronRunoff2Prec)
    yMiHuronOutflow1PP[jp] ~ dnorm(yMiHuronOutflow1Mean[jp], yMiHuronOutflow1Prec)
    yMiHuronOutflow2PP[jp] ~ dnorm(yMiHuronOutflow2Mean[jp], yMiHuronOutflow2Prec)
    yMiHuronDiversion1PP[jp] ~ dnorm(yMiHuronDiversion1Mean[jp], yMiHuronDiversion1Prec)

    # MONTH BY MONTH CHANGE IN STORAGE ANALYSIS

    ySuperiorDStorePP[jp] ~ dnorm(superiorDStore[jp], ySuperiorRStorePrec)

    superiorDStore[jp] <- (
        superiorPrecip[jp]
        -superiorEvap[jp]
        +superiorRunoff[jp]
        -superiorOutflow[jp]
        +superiorDiversion[jp]
        +superiorProcError[m[jp]]
    )

    yMiHuronDStorePP[jp] ~ dnorm(miHuronDStore[jp], yMiHuronRStorePrec)

    miHuronDStore[jp] <- (
        miHuronPrecip[jp]
        -miHuronEvap[jp]
        +miHuronRunoff[jp]
        +0.70110653739*superiorOutflow[jp]
```

```
        -miHuronOutflow[jp]
        -miHuronDiversion[jp]
        +miHuronProcError[m[jp]]
    )
}



### ROLLING SUM STORAGE ANALYSIS

# 1 YEAR

for(x in 12:posteriorEndMonth){
    ySuperiorR1YStorePP[x] ~ dnorm(superiorR1YStore[x], ySuperiorRStorePrec)

    superiorR1YStore[x] <- (
        sum(superiorPrecip[(x-12+1):x])
        -sum(superiorEvap[(x-12+1):x])
        +sum(superiorRunoff[(x-12+1):x])
        -sum(superiorOutflow[(x-12+1):x])
        +sum(superiorDiversion[(x-12+1):x])
        +sum(superiorProcError[m[(x-12+1):x]])
    )

    yMiHuronR1YStorePP[x] ~ dnorm(miHuronR1YStore[x], yMiHuronRStorePrec)

    miHuronR1YStore[x] <- (
        sum(miHuronPrecip[(x-12+1):x])
        -sum(miHuronEvap[(x-12+1):x])
        +sum(miHuronRunoff[(x-12+1):x])
        +0.70110653739*sum(superiorOutflow[(x-12+1):x])
        -sum(miHuronOutflow[(x-12+1):x])
        -sum(miHuronDiversion[(x-12+1):x])
        +sum(miHuronProcError[m[(x-12+1):x]])
    )
}

# 5 YEAR

for(z in 60:posteriorEndMonth){
    ySuperiorR5YStorePP[z] ~ dnorm(superiorR5YStore[z], ySuperiorRStorePrec)

    superiorR5YStore[z] <- (
        sum(superiorPrecip[(z-60+1):z])
        -sum(superiorEvap[(z-60+1):z])
        +sum(superiorRunoff[(z-60+1):z])
        -sum(superiorOutflow[(z-60+1):z])
        +sum(superiorDiversion[(z-60+1):z])
        +sum(superiorProcError[m[(z-60+1):z]])
    )

    yMiHuronR5YStorePP[z] ~ dnorm(miHuronR5YStore[z], yMiHuronRStorePrec)

    miHuronR5YStore[z] <- (
        sum(miHuronPrecip[(z-60+1):z])
        -sum(miHuronEvap[(z-60+1):z])
        +sum(miHuronRunoff[(z-60+1):z])
```

```
            +0.70110653739*sum(superiorOutflow[(z-60+1):z])
            -sum(miHuronOutflow[(z-60+1):z])
            -sum(miHuronDiversion[(z-60+1):z])
            +sum(miHuronProcError[m[(z-60+1):z]])
        )
    }

}

# END MODEL
```

```
### (f)12HH MODEL WITH POSTERIOR PREDICTIVE DISTRIBUTIONS FOR ALL VARIABLES

model {
    for (j in posteriorStartMonth:posteriorEndMonth){

        ##############################################
        ## Priors as described in section 2.2.2
        ## Model/Process errors follow equation set 5
        ## Data are fed in through R in jags.model
        ## function call, via data parameter
        ## Note: distribution parameters are
        ## mean and precision
        ## precision = 1/variance
        ##############################################

        ### SUPERIOR
        superiorPrecip[j] ~ dgamma(superiorPriorPrecipShape[m[j]], superiorPriorPrecipRate[m[j]])
        superiorEvap[j] ~ dnorm(superiorEvapPriorMean[m[j]], superiorEvapPriorPrecision[m[j]])
        superiorRunoff[j]   <- exp(superiorLogRunoff[j])
        superiorLogRunoff[j] ~ dnorm(superiorRunoffLogPriorMean[m[j]], superiorRunoffLogPriorPrecision[m[j]])
        superiorOutflow[j] ~ dnorm(superiorOutflowPriorMean[m[j]], superiorOutflowPriorPrecision[m[j]])
        superiorDiversion[j] ~ dnorm(superiorDiversionPriorMean[m[j]], superiorDiversionPriorPrecision[m[j]])
        superiorProcError_i[j] ~ dnorm(superiorProcError[m[j]], superiorProcError_iPrec[m[j]])

        ### MICHIGAN-HURON
        miHuronPrecip[j]    ~ dgamma(miHuronPriorPrecipShape[m[j]], miHuronPriorPrecipRate[m[j]])
        miHuronEvap[j] ~ dnorm(miHuronEvapPriorMean[m[j]], miHuronEvapPriorPrecision[m[j]])
        miHuronRunoff[j]    <- exp(miHuronLogRunoff[j])
        miHuronLogRunoff[j] ~ dnorm(miHuronRunoffLogPriorMean[m[j]], miHuronRunoffLogPriorPrecision[m[j]])
        miHuronOutflow[j] ~ dnorm(miHuronOutflowPriorMean[m[j]], miHuronOutflowPriorPrecision[m[j]])
        miHuronDiversion[j] ~ dnorm(miHuronDiversionPriorMean[m[j]], miHuronDiversionPriorPrecision[m[j]])
        miHuronProcError_i[j] ~ dnorm(miHuronProcError[m[j]], miHuronProcError_iPrec[m[j]])

        ########################################################
        ## Likelihood functions as described in section 2.2.2
        ## Biases follow equation set 7
        ########################################################

        ### SUPERIOR
        ySuperiorPrecip1[j] ~ dnorm(ySuperiorPrecip1Mean[j], ySuperiorPrecip1Prec)
        ySuperiorPrecip2[j] ~ dnorm(ySuperiorPrecip2Mean[j], ySuperiorPrecip2Prec)
        ySuperiorEvap1[j] ~ dnorm(ySuperiorEvap1Mean[j], ySuperiorEvap1Prec)
        ySuperiorEvap2[j] ~ dnorm(ySuperiorEvap2Mean[j], ySuperiorEvap2Prec)
        ySuperiorRunoff1[j] ~ dnorm(ySuperiorRunoff1Mean[j], ySuperiorRunoff1Prec)
        ySuperiorRunoff2[j] ~ dnorm(ySuperiorRunoff2Mean[j], ySuperiorRunoff2Prec)
        ySuperiorOutflow1[j]  ~ dnorm(ySuperiorOutflow1Mean[j], ySuperiorOutflow1Prec)
        ySuperiorOutflow2[j]  ~ dnorm(ySuperiorOutflow2Mean[j], ySuperiorOutflow2Prec)
        ySuperiorDiversion1[j]  ~ dnorm(ySuperiorDiversion1Mean[j], ySuperiorDiversion1Prec)

        ySuperiorPrecip1Mean[j] <- superiorPrecip[j] + ySuperiorPrecip1Bias_i[j]
        ySuperiorPrecip2Mean[j] <- superiorPrecip[j] + ySuperiorPrecip2Bias_i[j]
        ySuperiorEvap1Mean[j] <- superiorEvap[j] + ySuperiorEvap1Bias_i[j]
        ySuperiorEvap2Mean[j] <- superiorEvap[j] + ySuperiorEvap2Bias_i[j]
        ySuperiorRunoff1Mean[j] <- superiorRunoff[j] + ySuperiorRunoff1Bias_i[j]
        ySuperiorRunoff2Mean[j] <- superiorRunoff[j] + ySuperiorRunoff2Bias_i[j]
        ySuperiorOutflow1Mean[j] <- superiorOutflow[j] + ySuperiorOutflow1Bias_i[j]
        ySuperiorOutflow2Mean[j] <- superiorOutflow[j] + ySuperiorOutflow2Bias_i[j]
        ySuperiorDiversion1Mean[j] <- superiorDiversion[j] + ySuperiorDiversion1Bias_i[j]
```

```
    ySuperiorPrecip1Bias_i[j] ~ dnorm(ySuperiorPrecip1Bias[m[j]], ySuperiorPrecip1Bias_iPrec[m[j]]);
    ySuperiorPrecip2Bias_i[j] ~ dnorm(ySuperiorPrecip2Bias[m[j]], ySuperiorPrecip2Bias_iPrec[m[j]]);
    ySuperiorEvap1Bias_i[j] ~ dnorm(ySuperiorEvap1Bias[m[j]], ySuperiorEvap1Bias_iPrec[m[j]]);
    ySuperiorEvap2Bias_i[j] ~ dnorm(ySuperiorEvap2Bias[m[j]], ySuperiorEvap2Bias_iPrec[m[j]]);
    ySuperiorRunoff1Bias_i[j] ~ dnorm(ySuperiorRunoff1Bias[m[j]], ySuperiorRunoff1Bias_iPrec[m[j]]);
    ySuperiorRunoff2Bias_i[j] ~ dnorm(ySuperiorRunoff2Bias[m[j]], ySuperiorRunoff2Bias_iPrec[m[j]]);
    ySuperiorOutflow1Bias_i[j] ~ dnorm(ySuperiorOutflow1Bias[m[j]], ySuperiorOutflow1Bias_iPrec[m[j]]);
    ySuperiorOutflow2Bias_i[j] ~ dnorm(ySuperiorOutflow2Bias[m[j]], ySuperiorOutflow2Bias_iPrec[m[j]]);
    ySuperiorDiversion1Bias_i[j]~dnorm(ySuperiorDiversion1Bias[m[j]],ySuperiorDiversion1Bias_iPrec[m[j]]);

    ### MICHIGAN-HURON
    yMiHuronPrecip1[j] ~ dnorm(yMiHuronPrecip1Mean[j], yMiHuronPrecip1Prec)
    yMiHuronPrecip2[j] ~ dnorm(yMiHuronPrecip2Mean[j], yMiHuronPrecip2Prec)
    yMiHuronEvap1[j] ~ dnorm(yMiHuronEvap1Mean[j], yMiHuronEvap1Prec)
    yMiHuronEvap2[j] ~ dnorm(yMiHuronEvap2Mean[j], yMiHuronEvap2Prec)
    yMiHuronRunoff1[j] ~ dnorm(yMiHuronRunoff1Mean[j], yMiHuronRunoff1Prec)
    yMiHuronRunoff2[j] ~ dnorm(yMiHuronRunoff2Mean[j], yMiHuronRunoff2Prec)
    yMiHuronOutflow1[j]  ~ dnorm(yMiHuronOutflow1Mean[j], yMiHuronOutflow1Prec)
    yMiHuronOutflow2[j]  ~ dnorm(yMiHuronOutflow2Mean[j], yMiHuronOutflow2Prec)
    yMiHuronDiversion1[j]  ~ dnorm(yMiHuronDiversion1Mean[j], yMiHuronDiversion1Prec)

    yMiHuronPrecip1Mean[j] <- miHuronPrecip[j] + yMiHuronPrecip1Bias_i[j]
    yMiHuronPrecip2Mean[j] <- miHuronPrecip[j] + yMiHuronPrecip2Bias_i[j]
    yMiHuronEvap1Mean[j] <- miHuronEvap[j] + yMiHuronEvap1Bias_i[j]
    yMiHuronEvap2Mean[j] <- miHuronEvap[j] + yMiHuronEvap2Bias_i[j]
    yMiHuronRunoff1Mean[j] <- miHuronRunoff[j] + yMiHuronRunoff1Bias_i[j]
    yMiHuronRunoff2Mean[j] <- miHuronRunoff[j] + yMiHuronRunoff2Bias_i[j]
    yMiHuronOutflow1Mean[j] <- miHuronOutflow[j] + yMiHuronOutflow1Bias_i[j]
    yMiHuronOutflow2Mean[j] <- miHuronOutflow[j] + yMiHuronOutflow2Bias_i[j]
    yMiHuronDiversion1Mean[j] <- miHuronDiversion[j] + yMiHuronDiversion1Bias_i[j]

    yMiHuronPrecip1Bias_i[j] ~ dnorm(yMiHuronPrecip1Bias[m[j]], yMiHuronPrecip1Bias_iPrec[m[j]]);
    yMiHuronPrecip2Bias_i[j] ~ dnorm(yMiHuronPrecip2Bias[m[j]], yMiHuronPrecip2Bias_iPrec[m[j]]);
    yMiHuronEvap1Bias_i[j] ~ dnorm(yMiHuronEvap1Bias[m[j]], yMiHuronEvap1Bias_iPrec[m[j]]);
    yMiHuronEvap2Bias_i[j] ~ dnorm(yMiHuronEvap2Bias[m[j]], yMiHuronEvap2Bias_iPrec[m[j]]);
    yMiHuronRunoff1Bias_i[j] ~ dnorm(yMiHuronRunoff1Bias[m[j]], yMiHuronRunoff1Bias_iPrec[m[j]]);
    yMiHuronRunoff2Bias_i[j] ~ dnorm(yMiHuronRunoff2Bias[m[j]], yMiHuronRunoff2Bias_iPrec[m[j]]);
    yMiHuronOutflow1Bias_i[j] ~ dnorm(yMiHuronOutflow1Bias[m[j]], yMiHuronOutflow1Bias_iPrec[m[j]]);
    yMiHuronOutflow2Bias_i[j] ~ dnorm(yMiHuronOutflow2Bias[m[j]], yMiHuronOutflow2Bias_iPrec[m[j]]);
    yMiHuronDiversion1Bias_i[j] ~ dnorm(yMiHuronDiversion1Bias[m[j]], yMiHuronDiversion1Bias_iPrec[m[j]]);

}
```

```
###################################################
# Water balance model as described in section 2.1
# Model/Process error follows equation set 5
###################################################

for(k in rollPeriod:posteriorEndMonth){
    ### SUPERIOR
    ySuperiorRStore[k] ~ dnorm(superiorRStore[k], ySuperiorRStorePrec)

    superiorRStore[k] <- (
        sum(superiorPrecip[(k-rollPeriod+1):k])
        -sum(superiorEvap[(k-rollPeriod+1):k])
        +sum(superiorRunoff[(k-rollPeriod+1):k])
        -sum(superiorOutflow[(k-rollPeriod+1):k])
        +sum(superiorDiversion[(k-rollPeriod+1):k])
        +sum(superiorProcError_i[(k-rollPeriod+1):k])
    )

    ### MICHIGAN-HURON
    yMiHuronRStore[k] ~ dnorm(miHuronRStore[k], yMiHuronRStorePrec)

    miHuronRStore[k] <- (
        sum(miHuronPrecip[(k-rollPeriod+1):k])
        -sum(miHuronEvap[(k-rollPeriod+1):k])
        +sum(miHuronRunoff[(k-rollPeriod+1):k])
        -sum(miHuronOutflow[(k-rollPeriod+1):k])
        +0.70110653739*sum(superiorOutflow[(k-rollPeriod+1):k])
        -sum(miHuronDiversion[(k-rollPeriod+1):k])
        +sum(miHuronProcError_i[(k-rollPeriod+1):k])
    )
}

##################################################################
## Bias terms, monthly bias precisions, process errors, and monthly
## process error precisions, equation sets 7 and 5 respectively.
## Includes incorporation of expert guidance on Q and D
## They would otherwise have the same bias definition as the other
## variables
##################################################################
for (i in 1:12){
    ySuperiorPrecip1Bias[i] ~ dnorm(0,0.01)
    ySuperiorPrecip2Bias[i] ~ dnorm(0,0.01)
    ySuperiorEvap1Bias[i] ~ dnorm(0,0.01)
    ySuperiorEvap2Bias[i] ~ dnorm(0,0.01)
    ySuperiorRunoff1Bias[i] ~ dnorm(0,0.01)
    ySuperiorRunoff2Bias[i] ~ dnorm(0,0.01)
    ySuperiorOutflow1Bias[i] ~ dnorm(0,0.25)
    ySuperiorOutflow2Bias[i] ~ dnorm(0,0.25)
    ySuperiorDiversion1Bias[i] ~ dnorm(0,0.25)

    yMiHuronPrecip1Bias[i] ~ dnorm(0,0.01)
    yMiHuronPrecip2Bias[i] ~ dnorm(0,0.01)
    yMiHuronEvap1Bias[i] ~ dnorm(0,0.01)
```

```
    yMiHuronEvap2Bias[i] ~ dnorm(0,0.01)
    yMiHuronRunoff1Bias[i] ~ dnorm(0,0.01)
    yMiHuronRunoff2Bias[i] ~ dnorm(0,0.01)
    yMiHuronOutflow1Bias[i] ~ dnorm(0,0.25)
    yMiHuronOutflow2Bias[i] ~ dnorm(0,0.25)
    yMiHuronDiversion1Bias[i] ~ dnorm(0,0.25)

    ySuperiorPrecip1Bias_iPrec[i] ~ dgamma(0.05,0.05);
    ySuperiorPrecip2Bias_iPrec[i] ~ dgamma(0.05,0.05);
    ySuperiorEvap1Bias_iPrec[i] ~ dgamma(0.05,0.05);
    ySuperiorEvap2Bias_iPrec[i] ~ dgamma(0.05,0.05);
    ySuperiorRunoff1Bias_iPrec[i] ~ dgamma(0.05,0.05);
    ySuperiorRunoff2Bias_iPrec[i] ~ dgamma(0.05,0.05);
    ySuperiorOutflow1Bias_iPrec[i] ~ dgamma(0.05,0.05);
    ySuperiorOutflow2Bias_iPrec[i] ~ dgamma(0.05,0.05);
    ySuperiorDiversion1Bias_iPrec[i] ~ dgamma(0.05,0.05);

    yMiHuronPrecip1Bias_iPrec[i] ~ dgamma(0.05,0.05);
    yMiHuronPrecip2Bias_iPrec[i] ~ dgamma(0.05,0.05);
    yMiHuronEvap1Bias_iPrec[i] ~ dgamma(0.05,0.05);
    yMiHuronEvap2Bias_iPrec[i] ~ dgamma(0.05,0.05);
    yMiHuronRunoff1Bias_iPrec[i] ~ dgamma(0.05,0.05);
    yMiHuronRunoff2Bias_iPrec[i] ~ dgamma(0.05,0.05);
    yMiHuronOutflow1Bias_iPrec[i] ~ dgamma(0.05,0.05);
    yMiHuronOutflow2Bias_iPrec[i] ~ dgamma(0.05,0.05);
    yMiHuronDiversion1Bias_iPrec[i] ~ dgamma(0.05,0.05);

    superiorProcError[i] ~ dnorm(0,0.01)
    miHuronProcError[i] ~ dnorm(0,0.01)

    superiorProcError_iPrec[i] ~ dgamma(0.05,0.05);
    miHuronProcError_iPrec[i] ~ dgamma(0.05,0.05);
}

##############################
## Precision for Observations
##############################

### SUPERIOR
ySuperiorRStorePrec   ~ dgamma(0.01,0.01)
ySuperiorPrecip1Prec  ~ dgamma(0.1,0.1)
ySuperiorPrecip2Prec  ~ dgamma(0.1,0.1)
ySuperiorEvap1Prec    ~ dgamma(0.1,0.1)
ySuperiorEvap2Prec    ~ dgamma(0.1,0.1)
ySuperiorRunoff1Prec  ~ dgamma(0.1,0.1)
ySuperiorRunoff2Prec  ~ dgamma(0.1,0.1)
ySuperiorOutflow1Prec ~ dgamma(0.1,0.1)
ySuperiorOutflow2Prec ~ dgamma(0.1,0.1)
ySuperiorDiversion1Prec ~ dgamma(0.1,0.1)

### MICHIGAN-HURON
yMiHuronRStorePrec ~ dgamma(0.01,0.01)
yMiHuronPrecip1Prec ~ dgamma(0.1,0.1)
yMiHuronPrecip2Prec ~ dgamma(0.1,0.1)
yMiHuronEvap1Prec ~ dgamma(0.1,0.1)
yMiHuronEvap2Prec ~ dgamma(0.1,0.1)
yMiHuronRunoff1Prec ~ dgamma(0.1,0.1)
```

```
yMiHuronRunoff2Prec ~ dgamma(0.1,0.1)
yMiHuronOutflow1Prec ~ dgamma(0.1,0.1)
yMiHuronOutflow2Prec ~ dgamma(0.1,0.1)
yMiHuronDiversion1Prec ~ dgamma(0.1,0.1)



################################################################
# Posterior predictive (PP) distributions for verification
################################################################

for(jp in posteriorStartMonth:posteriorEndMonth){
    ### SUPERIOR
    ySuperiorPrecip1PP[jp] ~ dnorm(ySuperiorPrecip1Mean[jp], ySuperiorPrecip1Prec)
    ySuperiorPrecip2PP[jp] ~ dnorm(ySuperiorPrecip2Mean[jp], ySuperiorPrecip2Prec)
    ySuperiorEvap1PP[jp] ~ dnorm(ySuperiorEvap1Mean[jp], ySuperiorEvap1Prec)
    ySuperiorEvap2PP[jp] ~ dnorm(ySuperiorEvap2Mean[jp], ySuperiorEvap2Prec)
    ySuperiorRunoff1PP[jp] ~ dnorm(ySuperiorRunoff1Mean[jp], ySuperiorRunoff1Prec)
    ySuperiorRunoff2PP[jp] ~ dnorm(ySuperiorRunoff2Mean[jp], ySuperiorRunoff2Prec)
    ySuperiorOutflow1PP[jp] ~ dnorm(ySuperiorOutflow1Mean[jp], ySuperiorOutflow1Prec)
    ySuperiorOutflow2PP[jp] ~ dnorm(ySuperiorOutflow2Mean[jp], ySuperiorOutflow2Prec)
    ySuperiorDiversion1PP[jp] ~ dnorm(ySuperiorDiversion1Mean[jp], ySuperiorDiversion1Prec)

    ### MICHIGAN-HURON
    yMiHuronPrecip1PP[jp] ~ dnorm(yMiHuronPrecip1Mean[jp], yMiHuronPrecip1Prec)
    yMiHuronPrecip2PP[jp] ~ dnorm(yMiHuronPrecip2Mean[jp], yMiHuronPrecip2Prec)
    yMiHuronEvap1PP[jp] ~ dnorm(yMiHuronEvap1Mean[jp], yMiHuronEvap1Prec)
    yMiHuronEvap2PP[jp] ~ dnorm(yMiHuronEvap2Mean[jp], yMiHuronEvap2Prec)
    yMiHuronRunoff1PP[jp] ~ dnorm(yMiHuronRunoff1Mean[jp], yMiHuronRunoff1Prec)
    yMiHuronRunoff2PP[jp] ~ dnorm(yMiHuronRunoff2Mean[jp], yMiHuronRunoff2Prec)
    yMiHuronOutflow1PP[jp] ~ dnorm(yMiHuronOutflow1Mean[jp], yMiHuronOutflow1Prec)
    yMiHuronOutflow2PP[jp] ~ dnorm(yMiHuronOutflow2Mean[jp], yMiHuronOutflow2Prec)
    yMiHuronDiversion1PP[jp] ~ dnorm(yMiHuronDiversion1Mean[jp], yMiHuronDiversion1Prec)

    # MONTH BY MONTH CHANGE IN STORAGE ANALYSIS

    ySuperiorDStorePP[jp] ~ dnorm(superiorDStore[jp], ySuperiorRStorePrec)

    superiorDStore[jp] <- (
        superiorPrecip[jp]
        -superiorEvap[jp]
        +superiorRunoff[jp]
        -superiorOutflow[jp]
        +superiorDiversion[jp]
        +superiorProcError_i[jp]
    )

    yMiHuronDStorePP[jp] ~ dnorm(miHuronDStore[jp], yMiHuronRStorePrec)

    miHuronDStore[jp] <- (
        miHuronPrecip[jp]
        -miHuronEvap[jp]
        +miHuronRunoff[jp]
        +0.70110653739*superiorOutflow[jp]
        -miHuronOutflow[jp]
        -miHuronDiversion[jp]
```

```
        +miHuronProcError_i[jp]
    )
}




### CUMULATIVE STORAGE ANALYSIS

# 1 YEAR

for(x in 12:posteriorEndMonth){
    ySuperiorR1YStorePP[x] ~ dnorm(superiorR1YStore[x], ySuperiorRStorePrec)

    superiorR1YStore[x] <- (
        sum(superiorPrecip[(x-12+1):x])
        -sum(superiorEvap[(x-12+1):x])
        +sum(superiorRunoff[(x-12+1):x])
        -sum(superiorOutflow[(x-12+1):x])
        +sum(superiorDiversion[(x-12+1):x])
        +sum(superiorProcError_i[(x-12+1):x])
    )

    yMiHuronR1YStorePP[x] ~ dnorm(miHuronR1YStore[x], yMiHuronRStorePrec)

    miHuronR1YStore[x] <- (
        sum(miHuronPrecip[(x-12+1):x])
        -sum(miHuronEvap[(x-12+1):x])
        +sum(miHuronRunoff[(x-12+1):x])
        +0.70110653739*sum(superiorOutflow[(x-12+1):x])
        -sum(miHuronOutflow[(x-12+1):x])
        -sum(miHuronDiversion[(x-12+1):x])
        +sum(miHuronProcError_i[(x-12+1):x])
    )
}

# 5 YEAR

for(z in 60:posteriorEndMonth){
    ySuperiorR5YStorePP[z] ~ dnorm(superiorR5YStore[z], ySuperiorRStorePrec)

    superiorR5YStore[z] <- (
        sum(superiorPrecip[(z-60+1):z])
        -sum(superiorEvap[(z-60+1):z])
        +sum(superiorRunoff[(z-60+1):z])
        -sum(superiorOutflow[(z-60+1):z])
        +sum(superiorDiversion[(z-60+1):z])
        +sum(superiorProcError_i[(z-60+1):z])
    )

    yMiHuronR5YStorePP[z] ~ dnorm(miHuronR5YStore[z], yMiHuronRStorePrec)

    miHuronR5YStore[z] <- (
        sum(miHuronPrecip[(z-60+1):z])
```

```
            -sum(miHuronEvap[(z-60+1):z])
            +sum(miHuronRunoff[(z-60+1):z])
            +0.70110653739*sum(superiorOutflow[(z-60+1):z])
            -sum(miHuronOutflow[(z-60+1):z])
            -sum(miHuronDiversion[(z-60+1):z])
            +sum(miHuronProcError_i[(z-60+1):z])
        )
    }

}

# END MODEL
```
